# Supplementary material for: Identify As A Human Does: A Pathfinder of Next-Generation Anti-Cheat Framework for First-Person Shooter Games
Source: arXiv:2409.14830 source file (2025-11-17)
Supplement: Supplementary file 1 [file Robustness.tex]

\section{Cyclical Workflow for Model Refinement and Robustness to Cheat Evolution}
\label{appx:robustness}
At present, the cheat developers will modify and camouflage their cheats on a timely basis to evade anti-cheat inspections.
Therefore, the cheat evolution describes the phenomenon of specific anti-cheating programs becoming less effective over time.
All rule-based anti-cheat (e.g., signature detection, process detection, etc.) can not circumvent the influences of cheat evolution.
However, \sys starts the analysis from the behavior, thus avoiding the above limitations.
As long as cheaters want to gain an advantage over the norm, they must be better than average in terms of behavioral data (i.e., features) to gain an illegitimate advantage.
Therefore, no matter how the cheats adapt, as long as the cheaters still want to win the game, there is no way to bypass the detection of \sys.
In order to further validate the robustness of \sys and each of the subsystems against cheat evolution, we conducted an additional ablated experiment on \textit{Aimbot} dataset.
Classified through date, the dataset was divided into partitions (40 \textit{matches} per partition) containing variant cheat samples that adapted the official anti-cheat measures as time passed.
In \autoref{fig:robust_val} and \autoref{fig:robust_test} demonstrate the ablated different performance results of \sys across different numbers of partitions.
The ablated performance results of \sys on both sets have been fluctuating to maintain within a small range over partitions (time) and with the cheat evolution.
Thus it can be shown that \sys is robust to cheat evolution.
\input{Tables/expert skill levels}
\begin{figure}[htbp]
\centering
\includegraphics[width=0.47\textwidth]{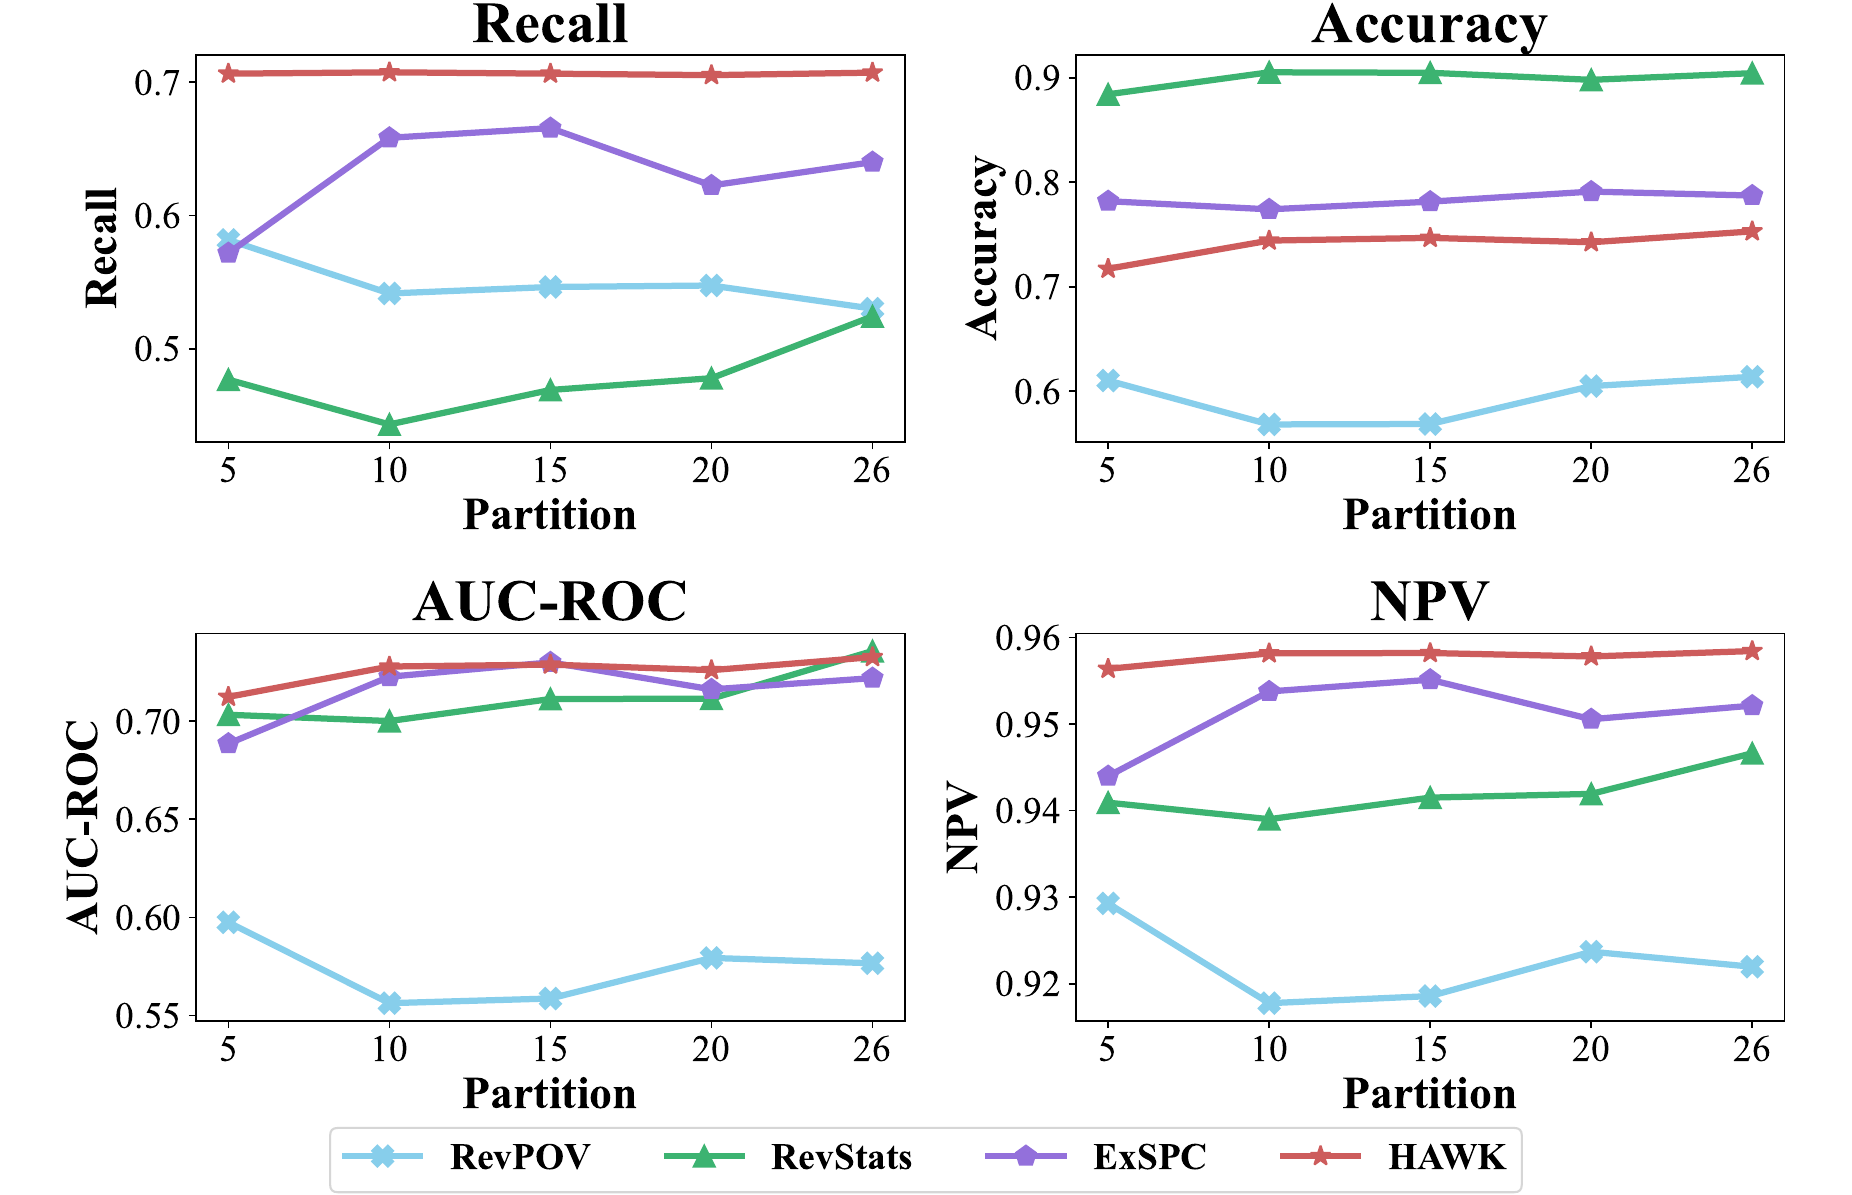}
\caption{Ablated Robustness on \textit{Aimbot} Validation Set}
\Description{Ablated Robustness on \textit{Aimbot} Validation Set}
\label{fig:robust_val}
\end{figure}
\begin{figure}[htbp]
\centering
\includegraphics[width=0.47\textwidth]{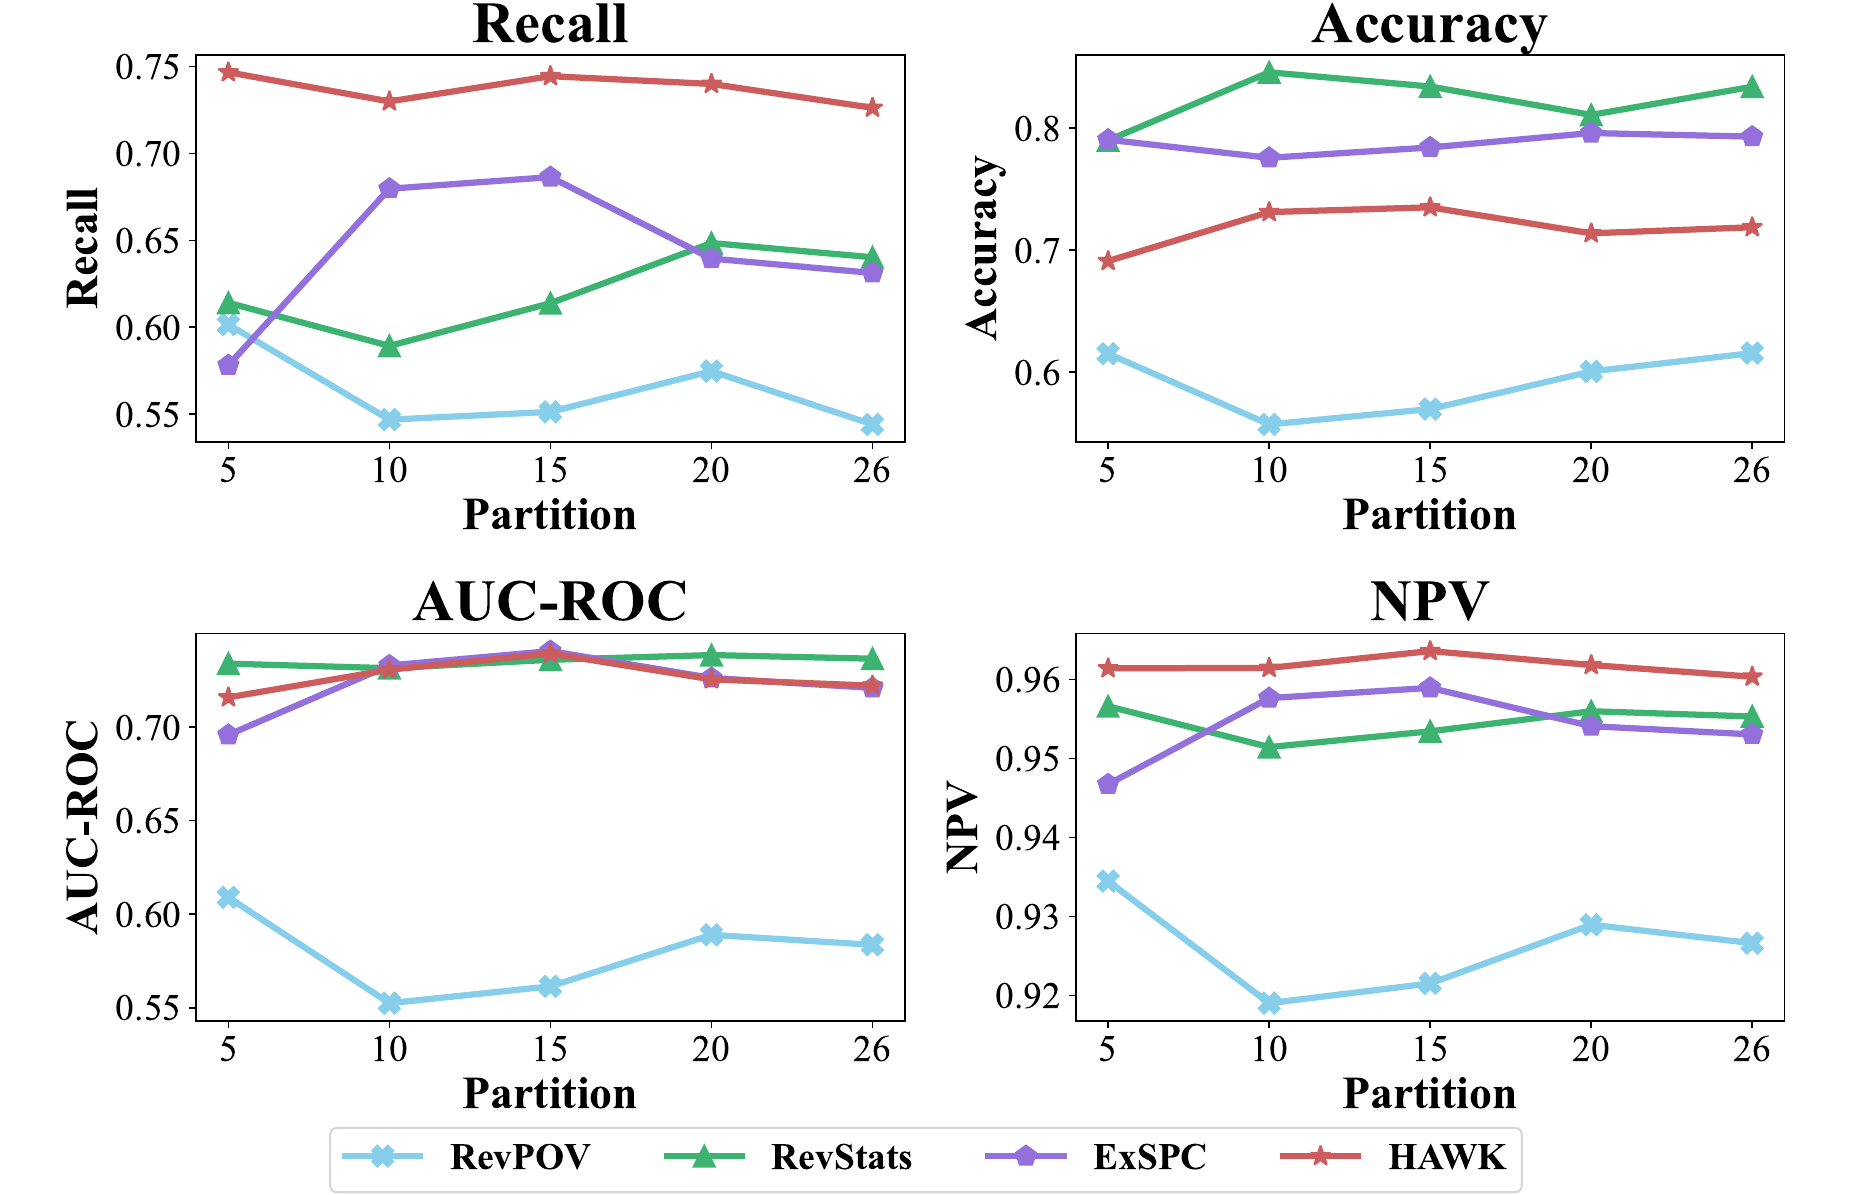}
\caption{Ablated Robustness on \textit{Aimbot} Test Set}
\Description{Ablated Robustness on \textit{Aimbot} Test Set}
\label{fig:robust_test}
\end{figure}
