# Supplementary material for: Identify As A Human Does: A Pathfinder of Next-Generation Anti-Cheat Framework for First-Person Shooter Games
Source: arXiv:2409.14830 source file (2025-11-17)
Supplement: Supplementary file 2 [file Evaluation_Metrics.tex]

\subsection{Evaluation Metrics} \label{app:evaluation}

\Jiayi{Cut down the words.}

% To set the stage for our detailed evaluation, here are some basic concepts pivotal in detecting cheating behaviors in FPS games. The forthcoming metrics, rooted in these elementary notions, will provide a lens through which we scrutinize the models' adeptness at identifying cheating instances amid the complex gaming environment.

% \textbf{True Positives (TP)}, shown in Eq.\ref{eq:TP}, represents instances where the model accurately predicts the occurrence of cheating behavior.

% \begin{equation}\label{eq:TP}
% TP = \sum_{i=1}^{n} I(y_i = 1 \land \hat{y}_i = 1)
% \end{equation}

% \textbf{True Negatives (TN)}, represented in Eq.\ref{eq:TN}, denotes instances where the model correctly identifies the absence of cheating behavior.

% \begin{equation}\label{eq:TN}
% TN = \sum_{i=1}^{n} I(y_i = 0 \land \hat{y}_i = 0)
% \end{equation}

% \textbf{False Positives (FP)}, represented in Eq.\ref{eq:FP}, encompass instances where the model erroneously predicts the presence of cheating behavior.

% \begin{equation}\label{eq:FP}
% FP = \sum_{i=1}^{n} I(y_i = 0 \land \hat{y}_i = 1)
% \end{equation}

% \textbf{False Negatives (FN)}, represented in Eq.\ref{eq:FN}, are instances where the model inaccurately predicts the absence of cheating behavior.

% \begin{equation}\label{eq:FN}
% FN = \sum_{i=1}^{n} I(y_i = 1 \land \hat{y}_i = 0)
% \end{equation}
% In these equations, $y_i$ denotes the true label, $\hat{y}_i$ signifies the predicted label, and $I(\cdot)$ represents the indicator function.

% With these basic elements, here are some metrics that are used in the evaluation.

\textbf{Recall}, represented in Eq.\ref{eq:Recall}, measures the proportion of actual positive instances that were correctly identified by the model.

\begin{equation}\label{eq:Recall}
Recall = \frac{TP}{TP + FN}
\end{equation}

\textbf{Accuracy}, as shown in Eq.\ref{eq:Accuracy}, gives a holistic measure of the model's performance across both positive and negative classes.

\begin{equation}\label{eq:Accuracy}
Accuracy = \frac{TP + TN}{TP + TN + FP + FN}
\end{equation}

% \textbf{Specificity}, illustrated in Eq.\ref{eq:Specificity}, computes the proportion of actual negative instances that were correctly identified by the model.

% \begin{equation}\label{eq:Specificity}
% Specificity = \frac{TN}{TN + FP}
% \end{equation}

% \textbf{Balanced Accuracy}, depicted in Eq.\ref{eq:BalancedAccuracy}, is the arithmetic mean of the True Positive Rate (TPR) and the True Negative Rate (TNR), offering a balanced perspective of the model's performance across both classes.

% \begin{equation}\label{eq:BalancedAccuracy}
% BA = \frac{TPR + TNR}{2}
% \end{equation}

\textbf{AUC-ROC}, denoted in Eq.\ref{eq:AUC-ROC}, is the area under the receiver operating characteristic curve, indicating the model's capability to differentiate between positive and negative classes. It is computed by integrating the ROC curve, as shown below:

\begin{equation}\label{eq:AUC-ROC}
AUC-ROC = \int_{0}^{1} TPR(FPR) \, dFPR
\end{equation}

where \( TPR \) (True Positive Rate) is synonymous with Recall, and \( FPR \) (False Positive Rate) is defined as \( \frac{FP}{FP + TN} \).

\textbf{NPV}, shown in Eq.\ref{eq:NPV}, is the proportion of actual negative instances among all instances predicted as negative.

\begin{equation}\label{eq:NPV}
NPV = \frac{TN}{TN + FN}
\end{equation}

% Lastly, \textbf{Informedness}, represented in Eq.\ref{eq:Informedness}, encapsulates the excess of true positive rate over false positive rate, offering a single-value summary of the model's diagnostic ability.

% \begin{equation}\label{eq:Informedness}
% Informedness = Recall + Specificity - 1
% \end{equation}

\textbf{Operational Efficiency Index (OEI)}, represented in Eq.\ref{eq:OEI}, is thus designed to encapsulate these conditions, offering a metric that reflects the operational efficiency gains in manual review processes. 

\begin{equation}\label{eq:OEI}
OEI = \left(\frac{N}{TP + FP}\right) \cdot (Recall \cdot NPV)
\end{equation}

Where, \(N\) represents the total number of all players. The \textit{OEI} metric encapsulates the diminution in manual review workload by refining the player pool requiring manual inspection, whilst upholding a high degree of rigor in cheater identification via elevated values of \textit{Recall} and \textit{NPV}. This metric succinctly delineates our system's prowess in enhancing operational efficiency by alleviating manual review endeavors, without undermining the integrity of the cheat detection process. The formulation of \textit{OEI} quantifies the degree to which our system facilitates the contraction of the manual review scope whilst conforming to the stringent requisites of precise cheater identification.

% Collectively, these metrics furnish a comprehensive and robust framework for the assessment and juxtaposition of various machine-learning models' performance within the realm of cheat detection.
