# Supplementary material for: Identify As A Human Does: A Pathfinder of Next-Generation Anti-Cheat Framework for First-Person Shooter Games
Source: arXiv:2409.14830 source file (2025-11-17)
Supplement: Supplementary file 3 [file RevPOV_Model_Selection_Preliminary_Test.tex]

\subsection{\syspov and 
\sysstats Model Comparison and Selection}
\label{appx:RevPoV_model_selection}
To select the optimized model for \syspov, we conducted comparison experiments on \syspov.
%
% For the timeliness of some of the experiments, we use the latest batch of datasets (different from the preliminary experiments) in the main paper.
%
In \autoref{tb:pov}, we listed several promising or commonly-used models' results among hundreds for comparison analysis after exhaustive experiments on different model selections of \syspov. For some poorly performing models, the OEI metric is N/A because there are no TP or FP predictions.
\syspov outperforms these models by maintaining a balanced, consistent performance across different datasets, thereby demonstrating its reliability. 
The tree-based strong learning capability is leveraged by implementing the \textit{multi-forest} design in the \textbf{Final Determination} stage. 
The \textit{multi-subsampling} makes the model more robust and acquires more data from the honest players, as well as ensuring the balanced data scales for avoiding overfitting problems.
