# Supplementary material for: Identify As A Human Does: A Pathfinder of Next-Generation Anti-Cheat Framework for First-Person Shooter Games
Source: arXiv:2409.14830 source file (2025-11-17)
Supplement: Supplementary file 4 [file RevStats_Model_Selection.tex]

\subsection{\sysstats Model Comparison and Selection}
\label{appx:RevStats_model_selection}
Similarly, to select the optimized model for \sysstats, we conducted comparison experiments on \sysstats.
\autoref{tb:stats} shows the performance metrics of various classifiers across validation and test sets for \sysstats. 
In the \autoref{tb:stats}, different classifiers displayed varying degrees of efficiency in distinguishing between cheaters and non-cheaters. 
Among these classifiers, the RandomForest performs with a higher accuracy than other individual classifiers. 
Nonetheless, each classifier contributes unique strengths to the ensemble, enhancing the overall performance of the \sysstats subsystem.
The \sysstats subsystem outperforms any single classifier model regarding the balance between recall and accuracy. 
%
% Specifically, it achieved superior recall, AUC-ROC, and accuracy on the validation and test sets compared to most of the individual classifiers. 
%
This performance improvement attests to the strength of the ensemble method, which capitalizes on the strengths of each classifier while mitigating their weaknesses.
